# Supplementary material for: Approximation Algorithms for $\ell_0$-Low Rank Approximation
Source: arXiv:1710.11253 source file (2018-10-01)
Supplement: Supplementary file 1 [file Appendix.tex]

\section{Omitted Proofs for Real \boldmath$\ell_{0}$-rank-\boldmath$k$}\label{app:secOmittedProofs}

\subsection{Proof of Lemma~\ref{lem_SR}}
Let $Q^{(0)}$ be the set of columns $j$ with $U V_{:,j} = 0$, and let $R^{(0)} \overset{\text{def}}{=} [n] \setminus Q^{(0)}$. Let $S^{(0)}\overset{\text{def}}{=}[n]$,
$T^{(0)}\overset{\text{def}}{=}\emptyset$. We split the value $\mathrm{OPT}^{(k)}$ into $\mathrm{OPT}(S^{(0)},R^{(0)})\overset{\text{def}}{=}\lVert A_{S^{(0)},R^{(0)}} - UV_{S^{(0)},R^{(0)}} \rVert_{0}$
and $\mathrm{OPT}(S^{(0)},Q^{(0)})\overset{\text{def}}{=}\lVert A_{S^{(0)},Q^{(0)}} - UV_{S^{(0)},Q^{(0)}} \rVert_{0}=\lVert A_{S^{(0)},Q^{(0)}}\rVert_{0}$.

Suppose $\mathrm{OPT}(S^{(0)},R^{(0)})\geq|S^{(0)}||R^{(0)}|/(k+1)$.
Then, for any subset $J^{(k)}$ it follows that $\min_{Z}\lVert A - A_{S^{(0)},J^{(k)}}Z \rVert_{0}\leq|S^{(0)}||R^{(0)}|+\lVert A_{S^{(0)},Q^{(0)}}\rVert_{0}\leq(k+1)\mathrm{OPT}^{(k)}$.
Otherwise, there is a column $i^{(1)}$ such that $\big\Vert A_{S^{(0)},i^{(1)}} -  (UV)_{S^{(0)},i^{(1)}} \big\Vert _{0}\leq\mathrm{OPT}(S^{(0)},R^{(0)})/|R^{(0)}| \le \mathrm{OPT}^{(k)} / |R^{(0)}|$.

Let $T^{(1)}$ be the set of indices on which $(UV)_{S^{(0)},i^{(1)}}$
and $A_{S^{(0)},i^{(1)}}$ disagree, and similarly $S^{(1)}\overset{\text{def}}{=}S^{(0)}\backslash T^{(1)}$
on which they agree. Then we have $|T^{(1)}|\leq \mathrm{OPT}^{(k)} / |R^{(0)}|$. Hence, in the submatrix $T^{(1)} \times R^{(0)}$ the total error is at most $|T^{(1)}| \cdot |R^{(0)}| \le \mathrm{OPT}^{(k)}$.
Let $R^{(1)},D^{(1)}$ be a partitioning
of $R^{(0)}$ such that $A_{S^{(1)},j}$ is linearly dependent on
$A_{S^{(1)},i^{(1)}}$ iff $j\in D^{(1)}$. Then by selecting
column $A_{:,i^{(1)}}$ the incurred cost on matrix $S^{(1)}\times D^{(1)}$ is zero. 
For the remaining submatrix $S^{(\ell)}\times R^{(\ell)}$, we perform a recursive call of the algorithm.

We make at most $k$ recursive calls, on instances $S^{(\ell)}\times R^{(\ell)}$
for $\ell\in\{0,\ldots,k-1\}$. In the $\ell^{th}$ iteration, either
$\mathrm{OPT}(S^{(\ell)},R^{(\ell)})\geq|S^{(\ell)}||R^{(\ell)}|/(k+1-\ell)$
and we are done, or there is a column $i^{(\ell+1)}$ which partitions
$S^{(\ell)}$ into $S^{(\ell+1)},T^{(\ell+1)}$ and $R^{(\ell)}$
into $R^{(\ell+1)},D^{(\ell+1)}$ such that 
%\[
%|S^{(\ell+1)}|\geq m\cdot\prod_{i=0}^{\ell}\left(1-\tfrac{1}{k+1-i}\right)=\tfrac{k-\ell}{k+1}\cdot m
%\]
%and 
for every $j\in D^{(\ell)}$ the column $A_{S^{(\ell+1)},j}$
belongs to the span of $\{A_{S^{(\ell+1)},i^{(t)}}\}_{t=1}^{\ell+1}$.

Suppose we performed $k$ recursive calls. We show now that
the incurred cost in submatrix $S^{(k)}\times R^{(k)}$ 
is at most $\mathrm{OPT}(S^{(k)},R^{(k)})\leq\mathrm{OPT}^{(k)}$.
By construction, 
%we have $|S^{(k)}|\geq m/(k+1)$, 
the sub-columns
$\{A_{S^{(k)},i}\}_{i\in I^{(k)}}$ are linearly independent, 
where $I^{(k)}=\{i^{(1)},\dots,i^{(k)}\}$ is the set of the selected columns,
and $A_{S^{(k)},I^{(k)}}=(UV)_{S^{(k)},I^{(k)}}$.
Since $\mathrm{rank}(A_{S^{(k)},I^{(k)}})=k$, it follows that
$\mathrm{rank}(U_{S^{(k)},:})=k$, $\mathrm{rank}(V_{:,I^{(k)}})=k$ and
the matrix $V_{:,I^{(k)}}\in\mathbb{R}^{k\times k}$ is invertible.
Hence, for matrix $Z=(V_{:,I^{(k)}})^{-1}V_{:,R^{k}}$ we have
$\mathrm{OPT}(S^{(k)},R^{(k)})=\lVert A_{S^{k},R^{k}}-A_{S^{k},I^{k}}Z\rVert_{0}$.

The statement follows by noting that the recursive calls accumulate 
a total cost of at most $k\cdot\mathrm{OPT}^{(k)}$ in the submatrices
$T^{(\ell+1)}\times R^{(\ell)}$ for $\ell \in \{0,1,\ldots,k-1\}$, as well as cost at most $\mathrm{OPT}^{(k)}$ in submatrix $S^{(k)}\times R^{(k)}$.\qed

\subsection{Proof of Theorem~\ref{thm_L0rankK_k^2approx}}

We use an algorithm of Berman and Karpinski~\cite{bk02} (attributed also to Kannan in that paper) which given a matrix $U$ and a vector $b$ approximates $\min_x \|Ux-b\|_0$ in polynomial time.
Specifically, we use the following variant of this result established by Alon, Panigrahy, and Yekhanin~\cite{APY09}.

\begin{thm}\label{thm_kAppxAlg} \cite{APY09} %($k$-approximation of the $\ell_{0}$-rank-$k$ problem) 
	There is an algorithm that given $A\in\mathbb{R}^{m\times k}$
	and $b\in\mathbb{R}^{m}$ outputs in $O(m^{2}k^{\omega+1})$
	time a vector $z\in\mathbb{R}^{k}$ such that w.h.p.\ $\left\Vert Az-b\right\Vert _{0}\leq k\cdot\min_{x}\left\Vert Ax-b\right\Vert _{0}$.
\end{thm}

The existence of a subset $J^{*}$ of $k$ columns of $A$ and matrix 
$Z^* \in\mathbb{R}^{k\times n}$
with $\lVert A - A_{:,J^{*}}Z^* \rVert_{0}\leq(k+1)\mathrm{OPT}^{(k)}$
follows by Lemma \ref{lem_SR}. 
We enumerate all ${n \choose k}$ subsets $J^{(k)}$ of $k$ columns.
For each $J^{(k)}$, we split $\min_{Z}\lVert A_{:,J^{(k)}}Z-A\rVert _{0}=
\sum_{i=1}^{n}\min_{z^{(i)}}
\lVert A_{:,J^{(k)}}z^{(i)}-A_{:,i}\rVert _{0}$, and we run the algorithm from Theorem~\ref{thm_kAppxAlg} $n$ times, obtaining approximate solutions $\tilde z^{(1)},\ldots,\tilde z^{(n)}$ forming a matrix $\tilde Z$. We return the best solution $(A_{:,J^{(k)}},\tilde Z)$. 
This yields a $k(k+1)$-approximation.
%Note that when $J^{(k)} = J^*$ we have
%\begin{align*}
%  \lVert A_{:,J^{*}} \tilde Z-A\rVert _{0} 
%  = \sum_{i=1}^{n}
%\lVert A_{:,J^{*}} \tilde z^{(i)}-A_{:,i}\rVert _{0} 
%  &\le k \sum_{i=1}^{n}\min_{z^{(i)}}
%\lVert A_{:,J^{*}}z^{(i)}-A_{:,i}\rVert _{0}  \\
% &= k \min_Z \lVert A_{:,J^{*}} Z-A\rVert _{0}  \\
% & \le k(k+1) \mathrm{OPT}^{(k)},
%\end{align*}
%where we used the approximation guarantee of Theorem~\ref{thm_kAppxAlg} and our structural Lemma~\ref{lem_SR}.
The time bound $O(n^{k+1} m^2 k^{\omega+1})$ is immediate from Theorem~\ref{thm_kAppxAlg}. This proves Theorem~\ref{thm_L0rankK_k^2approx}.

%
%
%Hence, it suffices to enumerate all
%${n \choose k}$ subsets $J^{(k)}$ of $k$ columns, and select 
%the one that minimizes the expression 
%$\min_{Z}\lVert A_{:,J^{(k)}}Z-A\rVert _{0}=
%\sum_{i=1}^{n}\min_{z^{(i)}}
%\lVert A_{:,J^{(k)}}z^{(i)}-A_{:,i}\rVert _{0}$.
%The statement follows by applying Theorem~\ref{thm_kAppxAlg} 
%for every $z^{(i)}$, i.e. we compute for each $z^{(i)}$ 
%an $O(k)$-approximation in $O(m^{2}k^{\omega+1})$ time.\qed

\subsection{Proof of Theorem \ref{thm_manuscript}}

Let $\Delta = \min_{\textrm{rank}(B) = k} \|A-B\|_0$. We can assume we know $\Delta$, since there are only $mn+1$ possibilities
of $\Delta$, and we can run the following algorithm for each such possibility, obtaining a rank-$O(k \log m)$ solution,
and then outputting the solution found with the smallest cost. This can be 
further optimized by instead only forming $O(\log(mn))$
guesses of $\Delta$, one of which will be within a factor of $2$ of the true 
value of $\Delta$, and observing that the following
argument only needs to know $\Delta$ up to a factor of $2$. 

We start by defining the notion of approximate coverage, which is different than the corresponding notion in \cite{cgklpw17} for
$p \geq 1$, due to the fact that $\ell_0$-regression cannot be efficiently solved. Consequently, approximate coverage for $p = 0$ cannot be
efficiently tested, complicating the proof.
We say that a column $A_{:,i}$ is
approximately covered by a subset $S$ of $k$ column indices of $A$ if $\min_x \|A_{:,S}x-A_{:,i}\|_0 \leq \frac{100(k+1) \Delta}{n}$, where
$A_{:,S}$ denotes the $m \times k$ submatrix of $A$ indexed by columns in $S$.

\begin{lem}(Similar to Lemma 6 in \cite{cgklpw17}, but modified to use our Lemma \ref{lem_SR})\label{lem:cover}
	Suppose we select a subset $R$ of $2k$ uniformly random columns of $A$. 
	Then with probability at least $2/9$, $R$
	approximately covers at least a $1/10$ fraction of columns of $A$.
\end{lem}
\begin{proof}[Proof of Lemma~\ref{lem:cover}]
	To show this, as in \cite{cgklpw17},
	consider a uniformly random column index $i$ not in the set $R$, and let $T = R \cup \{i\}$. Let $\eta$ be the cost of the best rank-$k$
	approximation to $A_{:,T}$ in $\ell_0$-norm. Since $T$ is a uniformly 
	random subset of $2k+1$ columns of $A$,
	${\bf E}[\eta] \le \frac{(2k+1) \Delta}{n}$, and so by a Markov bound, with probability at least $9/10$,
	we have $\eta \leq \frac{10(2k+1)\Delta}{n}$. Let $\mathcal{E}_1$ 
	denote this event.
	
	By Lemma \ref{lem_SR}, there exists a subset $L$ of $k$ columns of $A_{:,T}$
	for which $\min_X \|A_{:,L}X-A_{:,T}\|_0 \leq (k+1)\eta$. 
	Since $i$ is uniformly random given the set $T$, 
	${\bf E}_i[\min_x \|A_{:,L}x-A_{:,i}\|_0] \leq \frac{(k+1) \eta}{2k+1}$. 
	Let $\mathcal{E}_2$ denote the event that 
	$\min_x \|A_{:,L}x-A_{:,i}\|_0 \leq \frac{10(k+1)\eta}{2k+1}$, so $\Pr[\mathcal{E}_2] \geq 9/10$.
	
	Further, as in \cite{cgklpw17}, let $\mathcal{E}_3$ be the event that 
	$i \notin L$. Since $T$ is a set of $2k+1$ uniformly random columns and 
	$i \in T$ is a uniformly random element, we have
	$\Pr[\mathcal{E}_3] \geq \frac{k+1}{2k} > 1/2$. As in \cite{cgklpw17}, $\Pr[\mathcal{E}_1 \wedge \mathcal{E}_2 \wedge \mathcal{E}_3] \geq 3/10$,
	and conditioned on $\mathcal{E}_1 \wedge \mathcal{E}_2 \wedge \mathcal{E}_3$,
	$$\min_x \|A_{:,R}x-A_{:,i}\|_0 \leq \min_x \|A_{:,L}x-A_{:,i}\|_0 \leq \frac{10(k+1) \eta}{2k+1} \leq \frac{100(k+1)\Delta}{n},$$
	where the first inequality uses that $L$ is a subset of $R$ given $\mathcal{E}_3$, and so the regression cost cannot decrease, while the
	second inequality uses the occurrence of $\mathcal{E}_2$ and the final inequality uses the occurrence of $\mathcal{E}_1$.
	
	As in \cite{cgklpw17}, if $Z_i$ is an indicator random variable indicating 
	if $i$ is approximately covered by $R$, and $Z = \sum_i Z_i$, then
	${\bf E}[Z] \geq \frac{3m}{10}$ and ${\bf E}[m-Z] \leq \frac{7m}{10}$. 
	By a Markov bound, $\Pr[m-Z \geq \frac{9m}{10}] \leq \frac{7}{9}$.
	So $R$ approximately covers a $1/10$ fraction of columns of $A$ with 
	probability at least $2/9$.
\end{proof}

Given Lemma \ref{lem:cover}, we now present our algorithm. As noted above, a key difference with the corresponding Algorithm 3 of
\cite{cgklpw17} for $\ell_p$ for $p \geq 1$, is that we cannot efficiently test if a column $i$ is approximately covered by a set $R$.
We will instead again make use of Theorem~\ref{thm_kAppxAlg}.
%Instead, we use an algorithm of Berman and Karpinski \cite{bk02} (attributed also to Kannan in that paper) which given an $m \times r$
%matrix $U$ and an $m \times 1$ vector $b$, is able to obtain an $(r+1)$-approximation to $\min_x \|Ux-b\|_0$ in $\poly(mr)$ time.
%The algorithm is randomized but one can assume it succeeds with probability $1-1/\poly(mn)$
%by independently repeating it $O(\log(nm))$ times and taking the best $x$ found. 

We relax the notion of approximately covered to the notion of 
{\it nearly approximately covered} as follows: we say that a column $A_{:,i}$
is nearly approximately covered by a subset $S$ of columns of $A$ if, 
upon running the approximation algorithm of Theorem~\ref{thm_kAppxAlg}, the
computed vector $x$ satisfies 
$\|A_{:,S}x-A_{:,i}\|_0 \leq \frac{100(k+1)^2 \Delta}{n}$. 
By the guarantee of Theorem~\ref{thm_kAppxAlg}, if $A_i$ is approximately
covered by $S$ then it is also w.h.p.\ nearly approximately covered.
%with probability $1-1/\poly(mn)$. 

By Lemma \ref{lem:cover}, the expected number of iterations of selecting $2k$ 
columns in our Algorithm \ref{alg:randomcolumns} 
until a $(1/10)$-fraction of columns are nearly approximately covered is $O(1)$. 
When we recurse on $A_{:,\overline{R}}$, as in
\cite{cgklpw17}, we again have cost at most $\Delta$. There will be $O(\log m)$ recursive calls and thus by a Markov bound
the algorithm will choose $O(k \log m)$ columns in total. Since the approximation algorithm of Theorem~\ref{thm_kAppxAlg} is polynomial time, our entire algorithm
is expected polynomial time. When the algorithm terminates, each column is nearly approximately covered by a column we have chosen, which implies
if $A_{:,S}$ is our output set of columns, then 
$\min_X \|A_{:,S}X - A\|_0 \leq n \cdot \frac{100(k+1)^2 \Delta}{n} = 
100 (k+1)^2 \Delta$, which
completes the proof. \qed

\begin{algorithm}[H]
	\begin{algorithmic}
		\REQUIRE An integer $k$, and a matrix $A$.
		\ENSURE $O(k \log m)$ columns of $A$ 
		\STATE \hspace*{-5mm} \SelectColumns($k, A$):
		\IF{number of columns of $A \le 2k$}
		\STATE return all the columns of $A$
		\ELSE
		\REPEAT
		\STATE Let $R$ be uniform at random $2k$ columns of $A$
		\UNTIL {at least $(1/10)$-fraction columns of $A$ are nearly approximately covered}
		\STATE Let $A_{\overline{R}}$ be the columns of $A$ not nearly approximately
		covered by $R$
		\STATE return $R \cup$ \SelectColumns($k, A_{\overline{R}}$)
		\ENDIF
	\end{algorithmic}
	\caption{\label{alg:randomcolumns} Selecting $O(k \log m)$ columns of $A$.}
\end{algorithm}

\subsection{Proof of Lemma~\ref{lem_lowerBound_L0rankK}}

Notice that the optimum cost is at most $n$, achieved by selecting 
$U=(I_{k\times k};\ 0_{n\times k})$
and $V=G_{k\times n}$.

It is well known that Gaussian matrices are invertible with probability 1, see e.g.\ \cite[Thm 3.3]{SST06}. 
%For completeness we state here a recent result proved by
%Sankar, Spielman, and Teng~\cite{SST06}.
%
%\begin{lem}\label{lem_invGRM} 
%	(Invertibility of Gaussian Matrices \cite[Theorem 3.3 ]{SST06}).
%	Let $M\in\mathbb{R}^{n\times n}$ be an arbitrary square matrix, and
%	let $A=M+G\in\mathbb{R}^{n\times n}$ be a matrix such that the entries
%	of matrix $G$ are sampled i.i.d. from standard Gaussian distribution
%	$N(0,1)$. Then, for any $\delta\in(0,1)$ it holds $Pr[\sigma_{n}(A)\leq\delta/(2.35\sqrt{n})]\leq\delta$.
%	In particular, matrix $A$ is invertible.
%\end{lem}
Hence, $G_{:,J^{(k)}}$ is a nonsingular matrix 
for every subset $J^{(k)}\subset[n]$ of size $k$.

We will show next that for any subset $J^{(k)}$ of $k$ columns 
the incurred cost is at least $(n-k)k \ge nk/2$.
Without loss of generality, the chosen columns $J^{(k)} = [k]$ are the first $k$ columns of $A$. Let $R = [2k]$ be the first $2k$ rows and $C = [n] \setminus J$ be the last $n-k$ columns. We bound 
$$\min_Z \nnzs{A - A_{:,[k]} Z} \ge \min_Z \nnzs{A_{R,C} - A_{R,[k]} Z} = \sum_{j \in C} \min_{z^{(j)}} \nnzs{A_{R,j} - A_{R,[k]} z^{(j)}}, $$ 
i.e., we ignore all rows and columns except $R$ and $C$. Consider any column $j \in C$. Since $A_{R,j} = (G_{:,j}, 0_{k})$ and $A_{R,[k]} = (G_{:,[k]}, I_{k \times k})$, for any vector $z \in \mathbb{R}^k$ we have
$$\nnzs{A_{R,j} - A_{R,J^{(k)}} z} = \nnzs{G_{:,j} - G_{:,[k]} z} + \nnzs{I_{k \times k} z} 
= \nnzs{G_{:,j} - G_{:,[k]} z} + \nnz{z}.$$
Let $\ell \Def \nnz{z}$. By symmetriy, without loss of generality we can assume that the first $\ell$ entries of $z$ are non-zero and the remaining entries are 0. Let $x \in \mathbb{R}^\ell$ be the vector containing the first $\ell$ entries of $z$. Then we have
$$\nnzs{A_{R,j} - A_{R,J^{(k)}} z} = \nnzs{G_{:,j} - G_{:,[\ell]} x} + \ell.$$

We consider w.l.o.g. the first $k$ columns of $A$,
and we construct the optimum matrix $Z$ that minimizes
$\lVert A_{:,1:k}Z - A \rVert_{0}$. Observe that it is 
optimal to set the first $k$ columns of $Z$ to $I_{k\times k}$,
and since $A_{2k+1:n,1:k}=0$ we can focus only on the submatrix
$A_{1:2k,k+1:n}=(G_{1:k,k+1:n}; 0_{k\times n-k})$.

Consider a column $A_{1:2k,j}$ for $j\in[k+1,n]$. Our goal is to find
a vector $v\in\mathbb{R}^k$ minimizing the objective function
$\Psi=\min_{v}\{\lVert v\rVert_{0}+\lVert G^{(k)}v-g\rVert_{0}\}$,
where $G^{(k)}\Def\{G_{1:k,1:k}\}$ and $g\Def G_{1:k,j}$.
It holds with probability $1$ that $G^{(k)}$ and $g$
do not have an entry equal to zero. Moreover, since $G^{(k)}$ is invertible
every row in $[G^{(k)}]^{-1}$ is non-zero, and thus with probability
$1$ a vector $v=[G^{(k)}]^{-1}g$ has entry equal to zero.

Let $v=(x;\ 0)$ be an arbitrary vector with $\lVert x\rVert_{1}=\ell$.
Let $G^{(\ell)}$ be a submatrix of $G^{(k)}$ induced by the first
$\ell$ columns. For every subset $S\subset[m]$ of $\ell$ rows the
corresponding submatrix $G_{S,:}^{(\ell)}$ has a full rank. Suppose
there is a subset $S$ such that for $G_{S,:}^{(\ell)}$ and $g_{S}$
there is a vector $x\in\mathbb{R}^{k}$ satisfying $G_{S,:}^{(\ell)}x=g_{S}$.
Since $G_{S,:}^{(\ell)}$ is invertible, the existence of $x$ implies
its uniqueness. On the other hand, for any row $i\in[m]\backslash S$
the probability of the event $G_{i,:}^{(\ell)}x=g_{i}$ is equals
to $0$. Since $G^{(k)}v=G^{(\ell)}x$ and there are finitely many possible 
subsets $S$ as above, i.e. ${m \choose \ell}\leq m^{\ell}$, by union bound 
it follows that $\lVert G^{(k)}v-g\rVert_{0}\geq k-\ell$.
Therefore, it holds that $\phi\geq k$.

The statement follows by noting that the total cost incurred by
$A_{:,1:k}$ and any $Z$ is lower bounded by
$(n-k)k+(n-k)=\left(1-k/n\right)(k+1)n$. \qed
